# Supplementary material for: Relation-Aware Meta-Learning for Zero-shot Sketch-Based Image Retrieval
Source: arXiv:2412.00120 source file (2024-11-28)
Supplement: Supplementary file 1 [file X_suppl.tex]

\clearpage
\setcounter{page}{1}
\maketitlesupplementary
\section{Approach}
\subsection{The relation-aware quadruplet loss}
As shown in Figure \ref{duibi}, triplet loss provides single direction. Due to the gap between the modalities, samples from the same class in both modalities are far apart. For triplet loss, if we choose a sample from one modality, the direction of back-propagation may lead the anchor to the other modality. However, for quadruplet loss, there are two directions from negative samples to positive samples. They help anchor samples to avoid moving in the direction of negative samples and to approach positive samples. In the quadruplet case, we use a negative sample from a different mode as the second negative pair. This sample is further away and provides information about another modality. Two samples from each of the two modalities help to find the class center. Compared to the triplet loss, our relation-aware quadruplet loss is more robust.
\begin{figure}[!h]
\centering
\includegraphics[width=3.3in,height=2.7in]{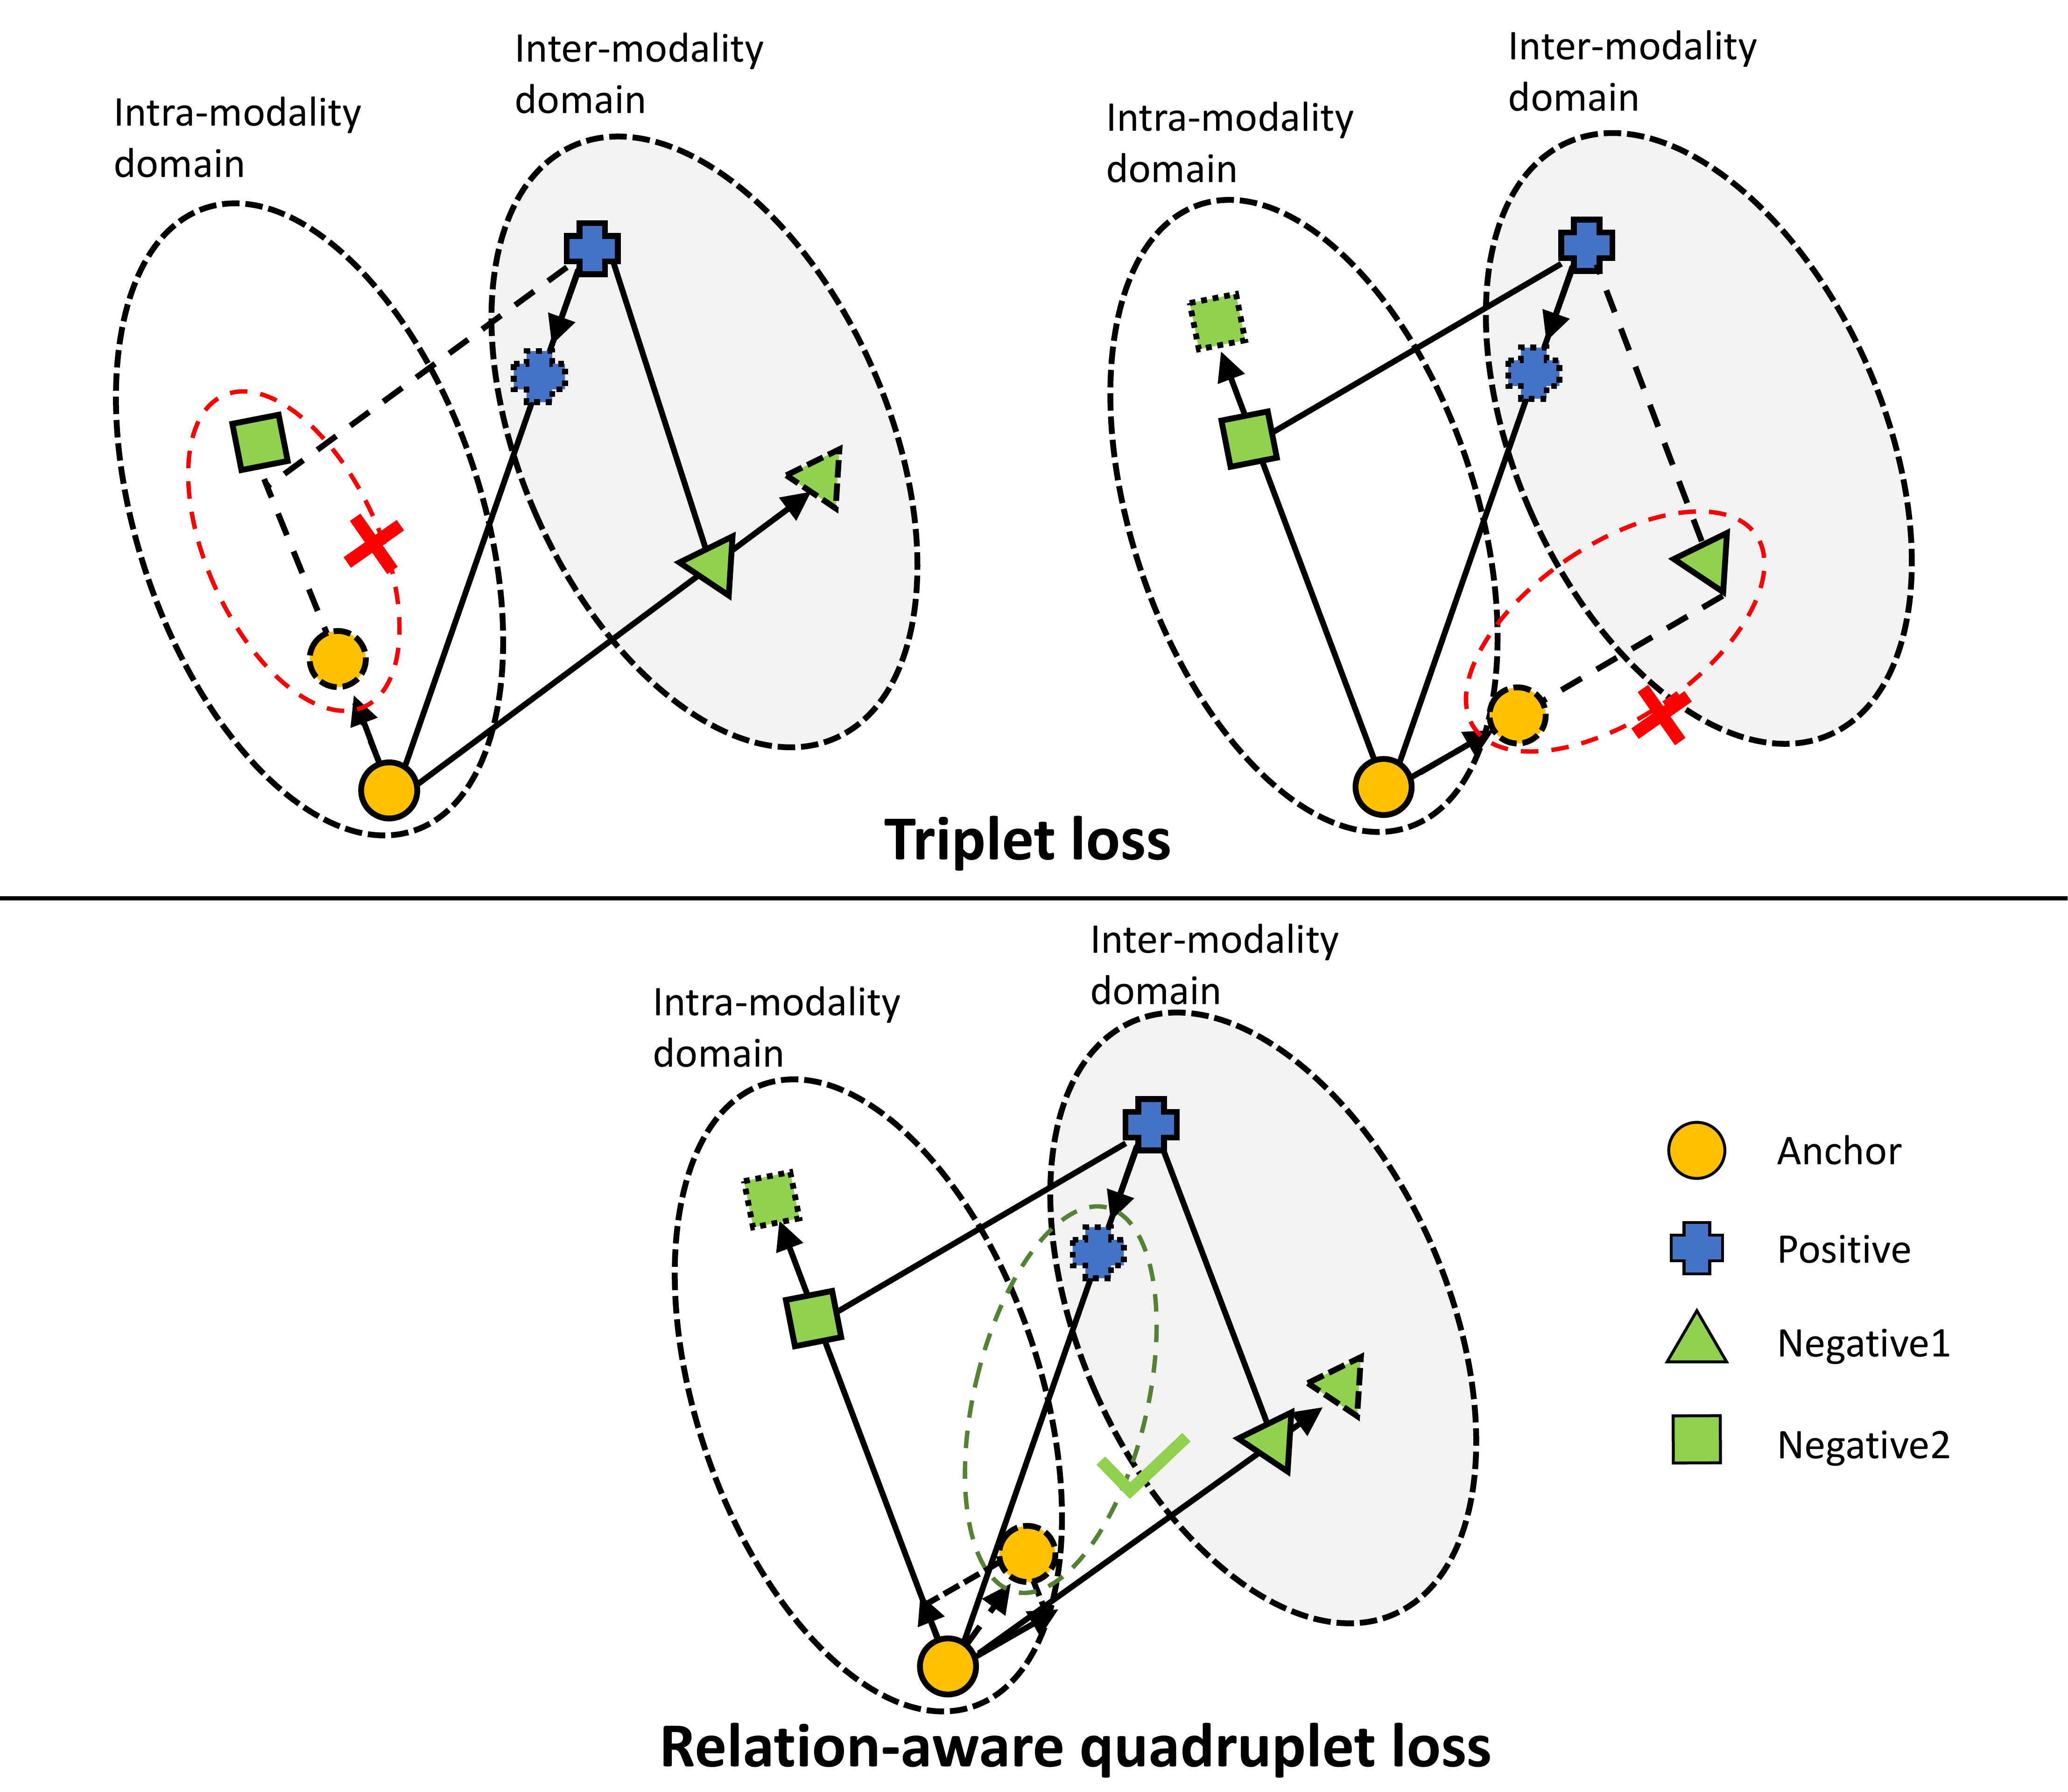}
\caption{In ZS-SBIR task, it is natural and reasonable to utilize samples from both modalities. However, how to balance them is a problem. On the one hand, considering the natural gap between modalities, increasing the distance effect is not effective; On the other hand,  pushing in the same modality may not make the anchor far away from the center of the negative class. }
\label{duibi}
\end{figure}
As shown in Figure \ref{intermodal}, the positive sample of global inter-modal quadruplet is in the same modality of the anchor image. It focuses on the entire embedding space and is suitable for the ZS-SBIR task. By reducing the intra-class distance from different modalities, the intra-class group is more compact: in ZS-SBIR, samples from the same class in the embedding space are always split into two parts due to natural differences between sketches and photos. Commonly, two parts are further apart than one part itself. So the main task in ZS-SBIR is to reduce the gap between sketch and photo. As shown in Figure \ref{intramodal}, for samples in the same modality, the distribution is still scattered and there are many outlier samples at the beginning of the training. Therefore, we use the local intra-modal quadruplet to enhance the compactness of two parts separately. Its positive images are in the same modality of the anchor. While pushing away the negative group, it helps two groups of the same class reduce their respective inter-class distances.

\begin{figure}[!t]
\centering
\includegraphics[width=3.2in,height=2.1in]{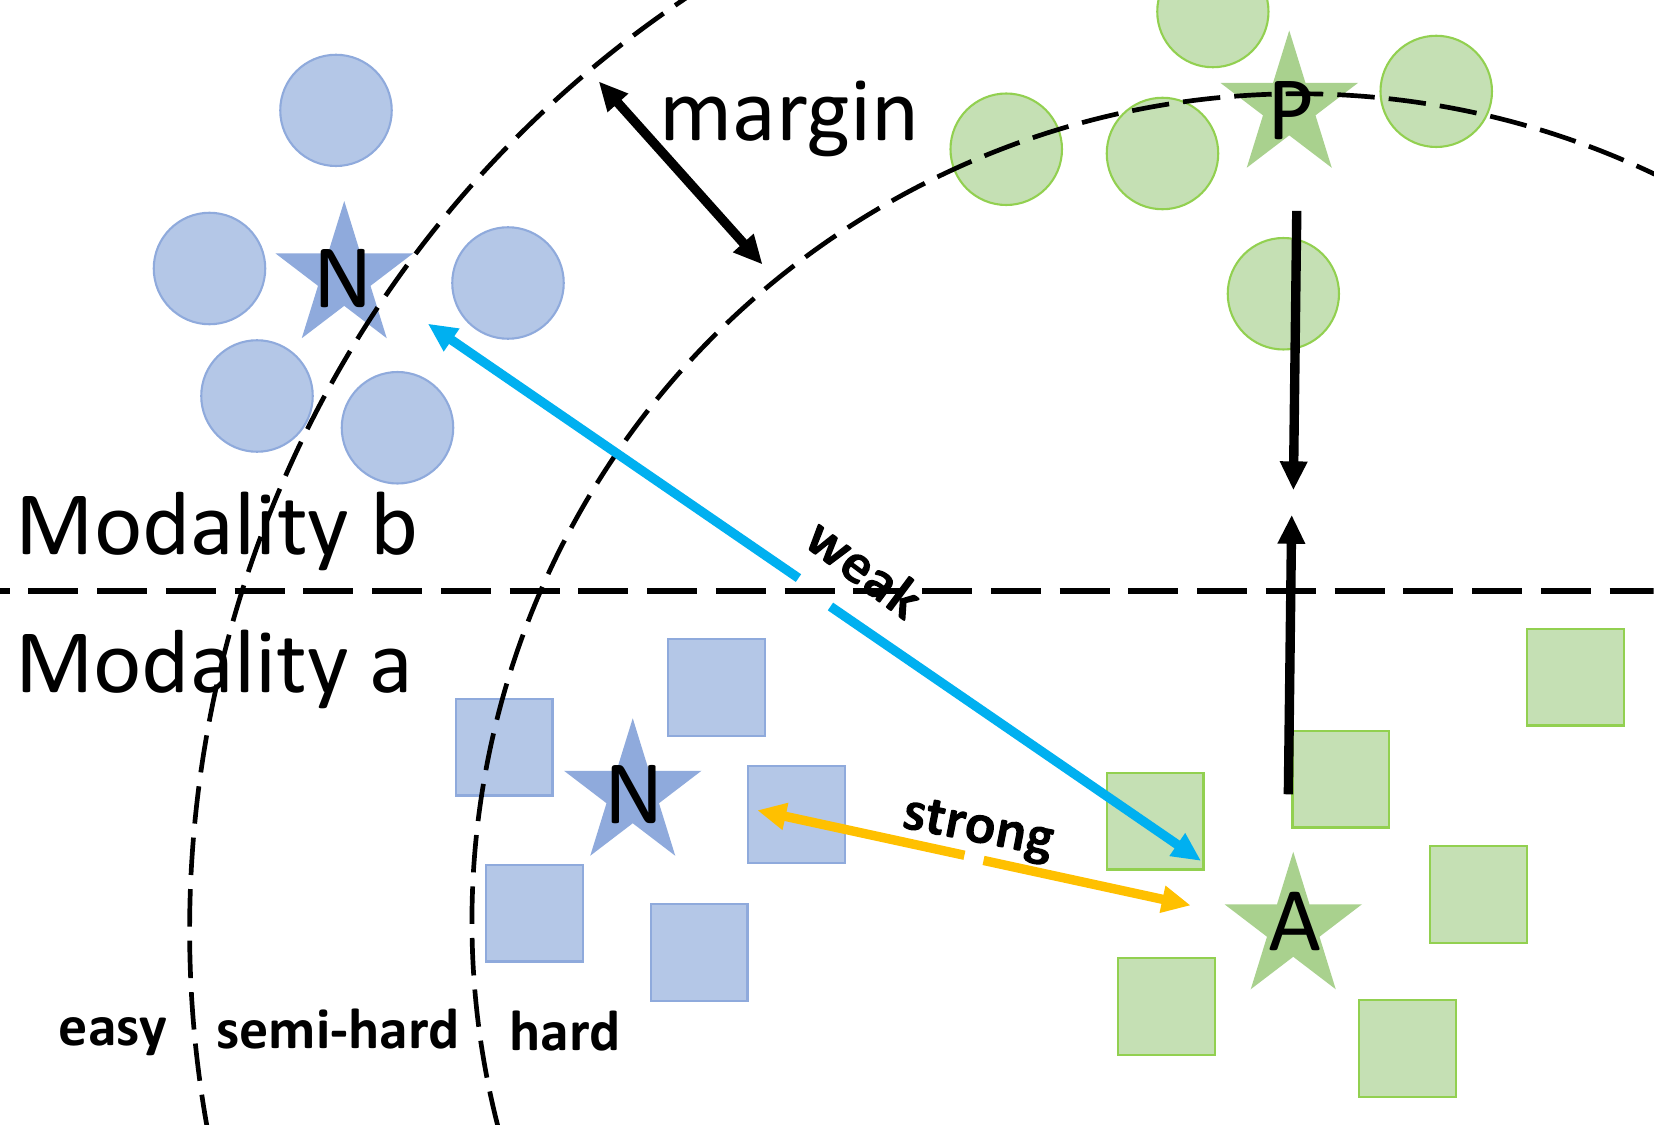}
\caption{Global inter-modal quadruplet. It makes two groups in the same class closer.}
\label{intermodal}
\end{figure}

\begin{figure}[!t]
\centering
\includegraphics[width=3.2in,height=2.1in]{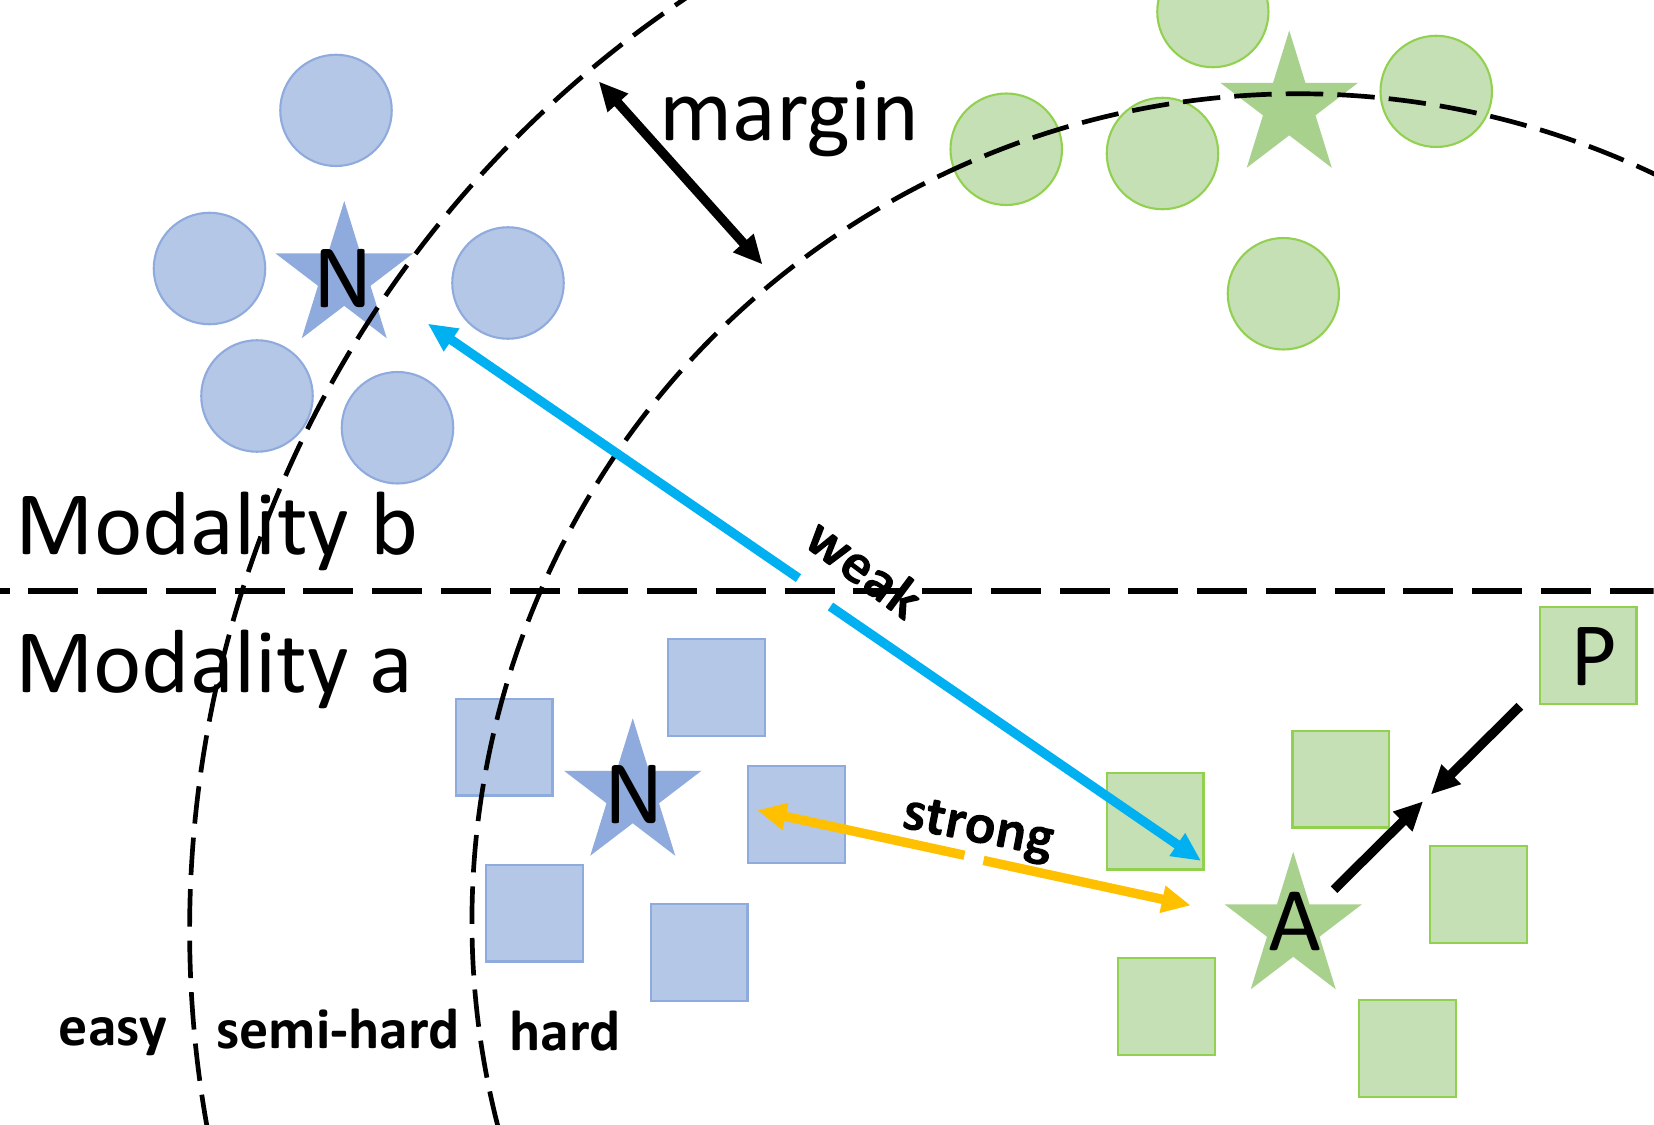}
\caption{Local intra-modal quadruplet. It searches for and closes outliers in the same modality}
\label{intramodal}
\end{figure}

\subsection{Meta Optimisation for the Loss Margin}
As shown in Figure \ref{meta}, we treat the input samples as a sequence, with the input denoted as $(x_{t}, l_{t-1})$, where $x$ represents the feature and $l$ represents the label. To prevent the network from directly associating features with labels and learning redundant positional information, we intentionally misalign the feature-label pairing. Subsequently, we utilize an external memory matrix to store the representations learned by the meta-learner (GRU). The GRU controller interacts with this external memory module through read and write heads. Given the feature input $x_{t}$, the GRU generates a key $k_{t}$, which is then stored in a row of the memory matrix. Finally, by calculating the distance between the key $k_{t}$ and the memory matrix, we enable both read and write operations. The procedure for writing feature vectors is as follows:
\begin{equation}\label{write}
\begin{split}
M_{t}(i)=M_{t-1}(i)+\textbf{w}_{t}^{w}(i)k_{t},
\end{split}
\end{equation}
where $M$ denotes the memory matrix used to store the learned representations, $M_{t-1}$ and $M_{t}$ represent the memory matrices at time steps $t-1$ and $t$, respectively. The write weight $w_{t}^{w}$ determines the positions in the memory matrix that should be written to. To extend the memory retention period, we prefer to write to the regions that have not been used recently. Therefore, the write weight is computed as follows:
\begin{equation}\label{weight}
\begin{split}
w_{t}^{w}= \alpha w_{t-1}^{r}+(1-\alpha)w_{t-1}^{lu},
\end{split}
\end{equation}
where $\alpha$ is a gating parameter, and $w_{t-1}^{lu}$ represents the least-used weights from the previous time step. These least-used weights are determined by comparing with the usage weights $w_{t}^{u}$:
\begin{equation}\label{weight-lu}
\begin{split}
\textbf{w}_{t}^{lu}(i)= \left\{\begin{array}{ll}
0 & \text { if } \textbf{w}_{t}^{u}(i)>m\left(w_{t}^{u}, n\right) \\
1 & \text { if } \textbf{w}_{t}^{u}(i) \leq m\left(w_{t}^{u}, n\right),
\end{array}\right.
\end{split}
\end{equation}
where $n$ is set to equal the number of reads to memory, and $m\left(w_{t}^{u}, n\right)$ denotes the $n$-th smallest value in the usage weight vector $w_{t}^{u}$.  This ensures that positions with lower usage weights are identified as least-used. The usage weights are updated at each time step by incorporating the previous usage weights along with the new read and write weights:
\begin{equation}\label{weight}
\begin{split}
w_{t}^{u}= w_{t-1}^{u}+w_{t}^{r}+w_{t}^{w},
\end{split}
\end{equation}
where $w_{t}^{r}$ are the read weights obtained by computing the dot product of the key $k_{t}$ and the memory through a Softmax function. When $w_{t}^{u}$ is less than $m\left(w_{t}^{u}, n\right)$, it indicates that position $i$ is among the least-used positions, thereby assigning higher write weights to it in the subsequent time step.

To read the content in memory matrix, we compute the cosine distance $D(k_{t}, M_{t}(i))$ between features $k_{t}$ and vectors in $M_{t}$. Then $D(k_{t}, M_{t}(i))$  is input to the Softmax function to obtain the read weights $w_{t}^{r}$. The final memory vector $m_{t}$ is obtained by weighted summation:
\begin{equation}\label{weight}
\begin{split}
m_{t} = \sum_{i} w_{t}^{r}(i) M_{t}(i).
\end{split}
\end{equation}
The matrix being read $m_{t}$ is used for margin $\mathcal{R}(x)$. Considering $\mathcal{L}_{ra-qua}$ contains $\mathcal{L}_{inter}$ and $\mathcal{L}_{intra}$, our method learns margin $\mathcal{R}(x)$ which has two values. Thus, We use a $(dim,2)$ linear layer with ReLU to obtain the margin. Learning two different margin helps $\mathcal{L}_{inter}$ and $\mathcal{L}_{intra}$ learn different relationship.

\begin{figure}[!t]
\centering
\includegraphics[width=3.2in,height=1.5in]{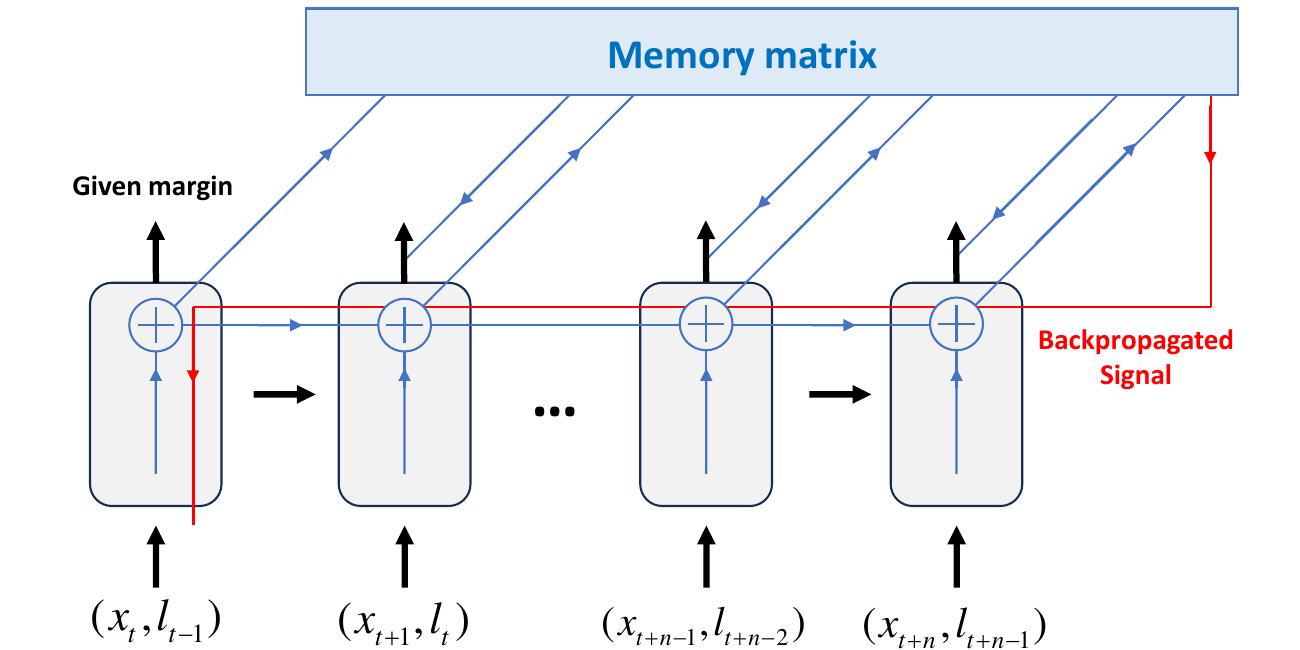}
\caption{ Meta optimisation for the loss Margin. We use an external memory matrix to record features obtained by meta learner (GRU), then the memory vector assists the current vector and gives a reasonable margin after subsequent operations. }
\label{meta}
\end{figure}

\section{Experiment}
\subsection{Ablation Study}
To demonstrate the effectiveness of our cross quadruplet approach, we created a series of triplet variants and conducted experiments on the TU-Berlin Extended dataset using CSE-ResNet as the backbone. We designed the following methods for comparison: a) The most common triplet \textbf{Com-Tri}, which exclusively selects the photo as the anchor. A positive distance is the distance between it and the same kind of sketch, and a negative distance is the distance between it and the non-kind sketch. b) Bidirectional triplet \textbf{Bid-Tri}. We add a set of triplets modally symmetric to Com-Tri: compute the distance between the sketch anchor and positive and negative photos. c) \textbf{All-Tri} Regardless of modality, only obtain triplets by class. This approach includes all possible combinations of triplets in both modality cases. d) Single quadruplet \textbf{Sin-Qua}. Our crossed quadruplets can be divided into two classes according to the positive pairs. \textbf{Sin-Qua} is one of two categories. If we remove $\mathcal{L}_{intra}(x,j,k)$ from Eq. \ref{quar}, we can get \textbf{Sin-Qua}, a formulation that includes solely cross-modality positive pairs. Detailed ablation study comparisons can be found in the ablation study section of the supplementary materials.

\textbf{Bid-Tri vs Com-Tri.}
For the ZS-SBIR task, it is normal to choose the sketch as the input for the anchor. In metric learning methods, they compute the distance as a similarity. The triplet that selects the sketch as an anchor can also adjust the distance between the sketch and the photo. Moreover, this triplet can be viewed as an object function that retrieves the sketch using a single photo. Thus, this objective function enhances the adaptability of the model to various retrieval tasks.

\textbf{Ra-Qua vs Sin-Qua.}
Another point of view is whether it is necessary to select inter-class images in the same modality as positive pairs. Since we need to compute distance across the modality, the distance is higher than that in the same modality. The loss could easily be lower than zero. However, our hard mining strategy only focuses on the maximum positive distance and the minimum negative distance. This strategy avoids ineffective training.

\textbf{Ra-Qua vs All-Tri.} As mentioned above, why not use all the positive types of triplets? Are all triplets helpful? In the section on relation-aware quadruplet loss, we have argued that distances across modalities are sufficient and we do not need to enhance them. Our relation-aware quadruplets use these secondary pairs to play their auxiliary role, preventing unwanted pushing and pulling from interfering with the model.

As shown in Figure.\ref{abl2}, our relation-aware quadruplet performs best. We would like to introduce our design ideas through comparison.

\begin{figure}[!h]
\centering
\includegraphics[width=3.4in,height=1.9in]{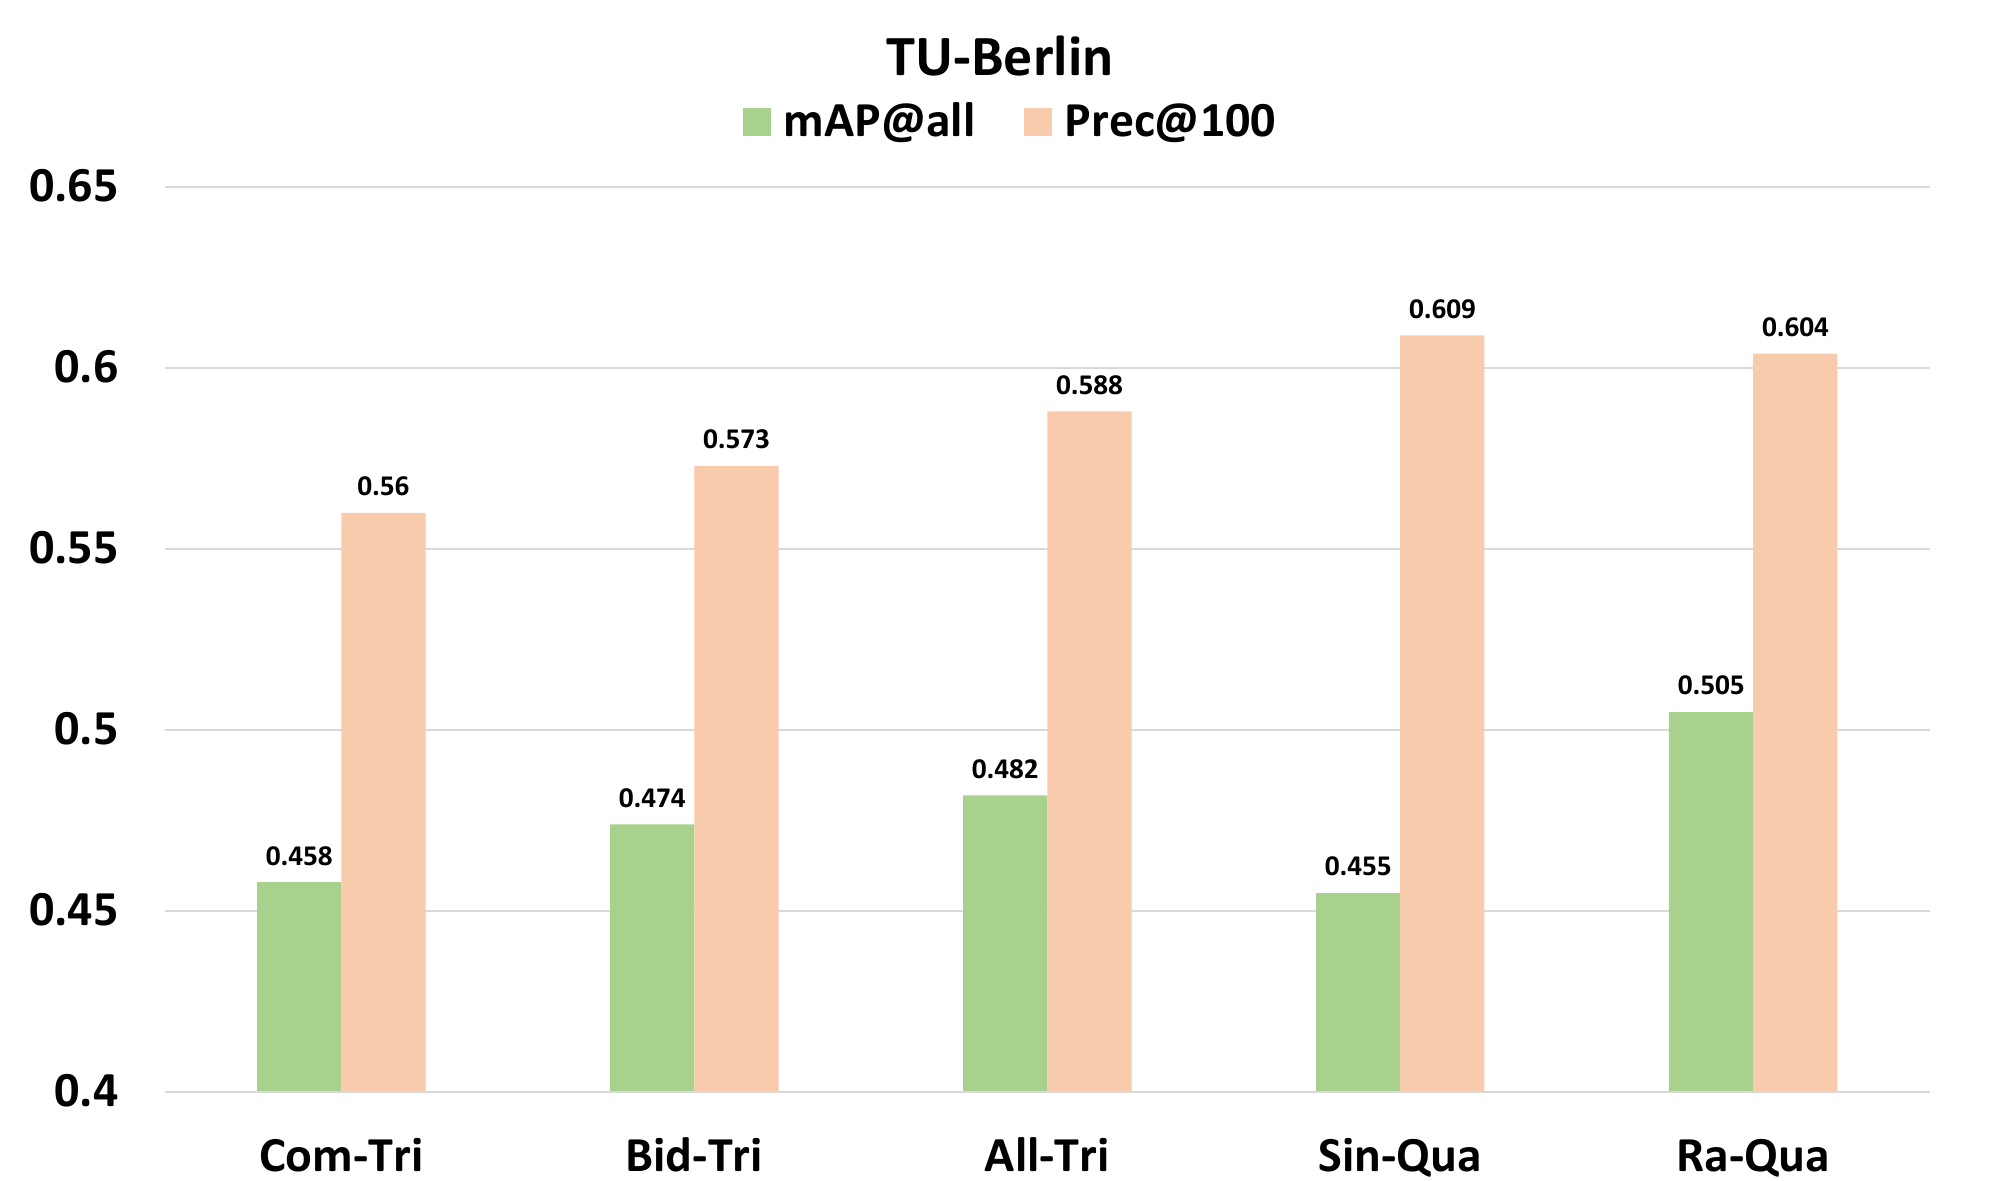}
\caption{Comparison of methods on TU-Berlin. The results in the table are all obtained without meta-learning. Our relation-aware quadruplet achieves best. Although the precision of \textbf{Sin-Qua} is slightly higher, its mAP is much lower.}
\label{abl2}
\end{figure}
\subsection{Visualization of Retrievals.}
To demonstrate the effectiveness of the proposed model more intuitively, we carefully select some examples of the top 7 retrieved candidates of sketch queries from the Sketchy dataset and compare them with the ZSE method \cite{lin2023zero}. As shown in Figure. \ref{visual-duibi}. Correct and incorrect candidates are marked with ticks and crosses, respectively. Numerous other sketches have also failed to be retrieved. Some classes share similar characteristics. For example, doors and windows have similar shapes and silhouettes and are hard to tell apart. But, compared to other existing methods, our method successfully retrieves some of the windows, which indicates that our method has more power to grasp the details of photos and sketches.
\begin{figure}[!h]
\centering
\hspace{-0.2cm}
\includegraphics[width=0.48\textwidth]{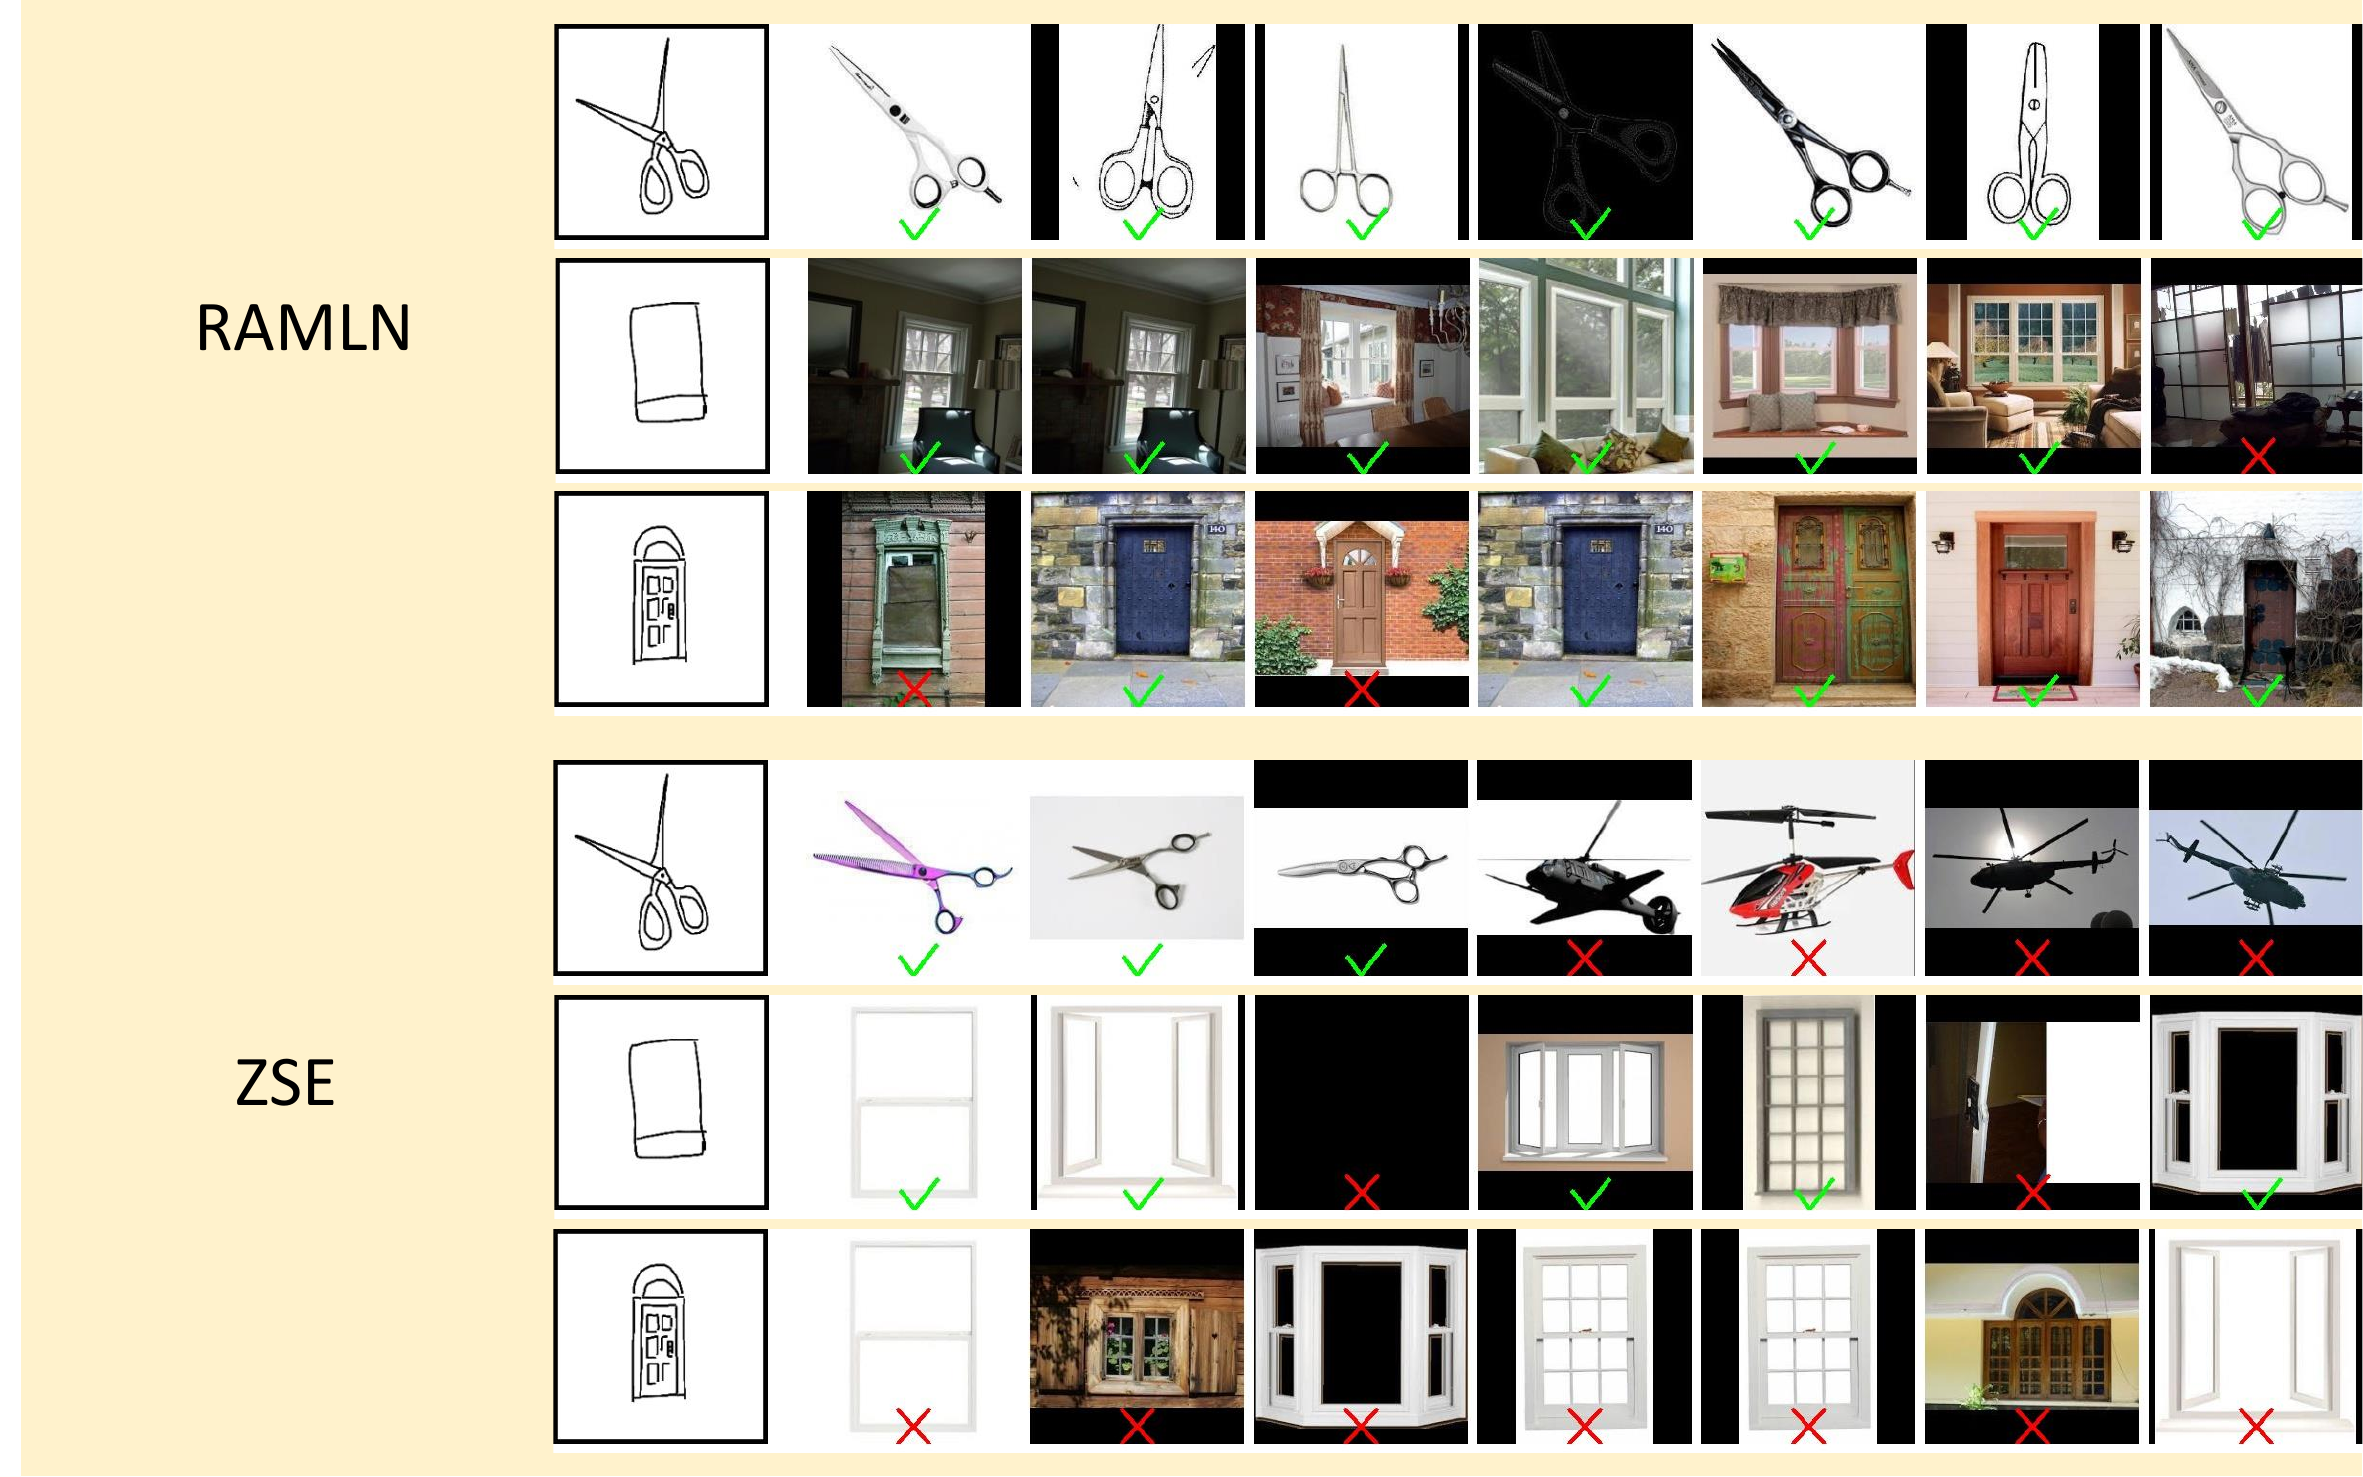}
\caption{We compare our methods with ZSE on Sketchy Ext.
There are instances where existing methods have failed to capture the nuances. For example, ZSE fails to tell the door and the window, whereas our model manages to retrieve some of these details successfully.
 }
\label{visual-duibi}
\end{figure}
